# Supplementary material for: Electric field tunable superconductor-semiconductor coupling in Majorana nanowires
Source: arXiv:1806.00988 ancillary file (2018-06-04)
Supplement: Supplementary file 1 [file Supplement.pdf]

# Supplemental information for "Electric field tunable superconductor-semiconductor coupling in Majorana nanowires"

Michiel W. A. de Moor,[1,*] Jouri D. S. Bommer,[1,*] Di Xu,[1,*] Georg W. Winkler,[2] Andrey E. Antipov,[2] Arno Bargerbos,[1] Guanzhong Wang,[1] Nick van Loo,[1] Roy L. M. Op het Veld,[1,3] Sasa Gazibegovic,[1,3] Diana Car,[1,3] John A. Logan,[4] Mihir Pendharkar,[5] Joon Sue Lee,[5] Erik P. A. M. Bakkers,[1,3] Chris J. Palmstrøm,[4,5] Roman M. Lutchyn,[2] Leo P. Kouwenhoven,[1,6] and Hao Zhang[1,†]

[1]*QuTech and Kavli Institute of NanoScience, Delft University of Technology, 2600 GA Delft, The Netherlands*

[2]*Station Q, Microsoft Research, Santa Barbara, California 93106-6105, USA*

[3]*Department of Applied Physics, Eindhoven University of Technology, 5600 MB Eindhoven, The Netherlands*

[4]*Materials Department, University of California, Santa Barbara, California 93106, USA*

[5]*Electrical and Computer Engineering, University of California, Santa Barbara, California 93106, USA*

[6]*Microsoft Station Q at Delft University of Technology, 2600 GA Delft, The Netherlands*

[*] These authors contributed equally to this work.

[†] H.Zhang-3@tudelft.nl

**CONTENTS**


S1. Simulation of electrostatics and nanowire spectrum 3

S2. Electric field dependence of spin-orbit coupling 5

S3. Simulated band structure 6

S4. Fabrication procedure 7

S5. Device information and schematics 8

S6. Gap fitting & additional data 9

S7. g-factor fitting & additional data 12

S8. Anticrossing fitting 15

S9. Simulation of finite size nanowire system 16

S10. Additional ZBP data 19

References 22

## S1. SIMULATION OF ELECTROSTATICS AND NANOWIRE SPECTRUM

For the electrostatics simulations we use the geometry of device A (as shown in Fig. 1(c) of the main text). We describe the device as an infinite wire oriented along the $x$-direction, with a hexagonal cross-section in the $yz$-plane. The electrostatics are described by the Poisson equation

$$\nabla \cdot (\epsilon_r(\mathbf{r}) \nabla \phi(\mathbf{r})) = \frac{\rho_{\mathrm{tot}}[\phi(\mathbf{r})]}{\epsilon_0}, \tag{S1}$$

where $\rho_{\mathrm{tot}}[\phi(\mathbf{r})]$ is a functional of the potential $\phi(\mathbf{r})$. We include four contributions to $\rho_{\mathrm{tot}}$,

$$\rho_{\mathrm{tot}} = \rho_{\mathrm{e}} + \rho_{\mathrm{hh}} + \rho_{\mathrm{lh}} + \rho_{\mathrm{fixed}}, \tag{S2}$$

where $\rho_{\mathrm{e}}$, $\rho_{\mathrm{hh}}$ and $\rho_{\mathrm{lh}}$ are the mobile charges of the conduction band, heavy hole band and light hole band of the InSb nanowire and $\rho_{\mathrm{fixed}}$ are the fixed charges in the system. For the mobile electron charges we assume a 3D electron gas density (Thomas-Fermi approximation)

$$\rho_{\mathrm{e}}(\phi) = -\frac{e}{3\pi^2} \left( \frac{2m_{\mathrm{e}}|\phi|\theta(-\phi)}{\hbar^2} \right)^{3/2}, \tag{S3}$$

with $\theta$ the Heaviside step function, and for the holes

$$\rho_i(\phi) = \frac{e}{3\pi^2} \left( \frac{2m_i|\phi - E_{\mathrm{G}}|\theta(\phi - E_{\mathrm{G}})}{\hbar^2} \right)^{3/2}, \tag{S4}$$

with $E_{\mathrm{G}}$ the band gap and $i$ corresponding to the heavy hole (hh) and light hole (lh) band respectively. For the effective masses, we take the bulk InSb values [1]. We include hole bands to describe the additional screening when the electrochemical potential is in the valence band, which can become relevant for very negative gate voltages due to the narrow band gap of InSb. To model the influence of the sputtered dielectric on the nanowire surface, the wire is wrapped in a 1 nm surface layer of $2.5 \times 10^{18}\,\mathrm{cm}^{-3}$ positive charge density. In the absence of other charges and gates this charge pins the conduction band of InSb at about -0.069 eV below the Fermi level at the surface. For the InSb-Al interface we assume the conduction band of InSb is pinned -0.08 eV below the Fermi level due to the work function difference between the two materials. A negative band offset of the semiconductor to the superconductor is required for a hard induced gap in the InAs-Al system [2], and we assume a similar situation in InSb-Al hybrid devices. While the precise numbers for the surface accumulation and band-offset at the InSb-Al interface are unknown, it is known that InSb wires have about a 10 times smaller density than InAs wires [3, 4], and the parameters were

**TABLE SI:** Material parameters for InSb and Al.

| Parameter | InSb | Al |
|---|---|---|
| $m^*$ | 0.0139 [1] | 1 |
| $g$ | -40 [5] | 2 |
| $\Delta$ | 0 meV | 0.34 meV [6] |
| $E_\mathrm{F}$ | 0 eV | 10 eV [7] |

adjusted from the InAs ones accordingly. The Al layer is assumed to be grounded, and enters as a Dirichlet boundary condition which is set to +0.08 V. The boundary condition at the substrate-dielectric interface is set to the applied gate voltage, $V_\mathrm{Gate}$. On the remaining three boundaries of the system we use Neumann conditions. For the dielectric constant of InSb, the sputtered $SiN_x$, and the LPCVD $Si_3N_4$ we take take 15.15, 7.5, and 8 respectively.

After the electrostatic potential has been calculated for a given $V_\mathrm{Gate}$, we plug it into the Schrödinger equation and solve it for the cross-section of the device. We use a Rashba Hamiltonian with a Bogoliubov-de Gennes (BdG) superconducting term [8]

$$\begin{aligned} H =& \frac{\hbar^2}{2m^*(y,z)}(k_x^2+k_y^2+k_z^2)\tau_z - (E_\mathrm{F}(y,z)+e\phi(y,z))\tau_z + \alpha_y(y,z)(k_z\sigma_x - k_x\sigma_z)\tau_z \\ &+ \alpha_z(y,z)(k_x\sigma_y - k_y\sigma_x)\tau_z + \frac{1}{2}g(y,z)\mu_\mathrm{B}B\sigma_x + \Delta(y,z)\tau_x, \end{aligned} \tag{S5}$$

where the effective mass $m^*$, the Fermi level $E_\mathrm{F}$, the electrostatic potential $\phi$, the Rashba parameters $\alpha_i$, the g-factor and the superconducting pairing $\Delta$ are functions of the $(y,z)$-coordinates and depend on the material. Since $\phi$ is not solved in Al it is correspondingly set to zero there. The material parameters for InSb and Al are summarized in Tab. SI. If desired, the orbital effect is added to Eq. (S5) by the Peierls substitution $k_z \to k_z - \frac{\pi}{\phi_0}B(y-y_0)$, with $\phi_0$ the magnetic flux quantum. $y_0$ is chosen such that the average vector potential in Al is zero, resulting in a vanishing supercurrent [9]. The Hamiltonian is discretised on a quadratic mesh and constructed using the `kwant` package [10]. To accommodate the small Fermi wavelength of Al a discretisation length of 0.1 nm is used.

## S2. ELECTRIC FIELD DEPENDENCE OF SPIN-ORBIT COUPLING

The Rashba couplings $\alpha_y$ and $\alpha_z$, which are nonzero only in the semiconductor region, result from the symmetry breaking by the electrostatic potential and are obtained from [1]

$$\alpha_i = \frac{eP^2}{3}\left[\frac{1}{E_0} - \frac{1}{(E_0+\Delta_0)^2}\right]\bar{\mathcal{E}}_i, \tag{S6}$$

where the average electric field in direction $i$ is obtained by averaging $\mathcal{E}_i$ over the whole semiconductor region. Parameters for bulk InSb are used [1]: the Kane matrix element $P = 0.9641\,\mathrm{eV\,nm}$, the bandgap $E_0 = 0.237\,\mathrm{eV}$, and the spin-orbit gap $\Delta_0 = 0.810\,\mathrm{eV}$. The resulting Rashba parameters $\alpha_i$ are plotted in Fig. S1(a).

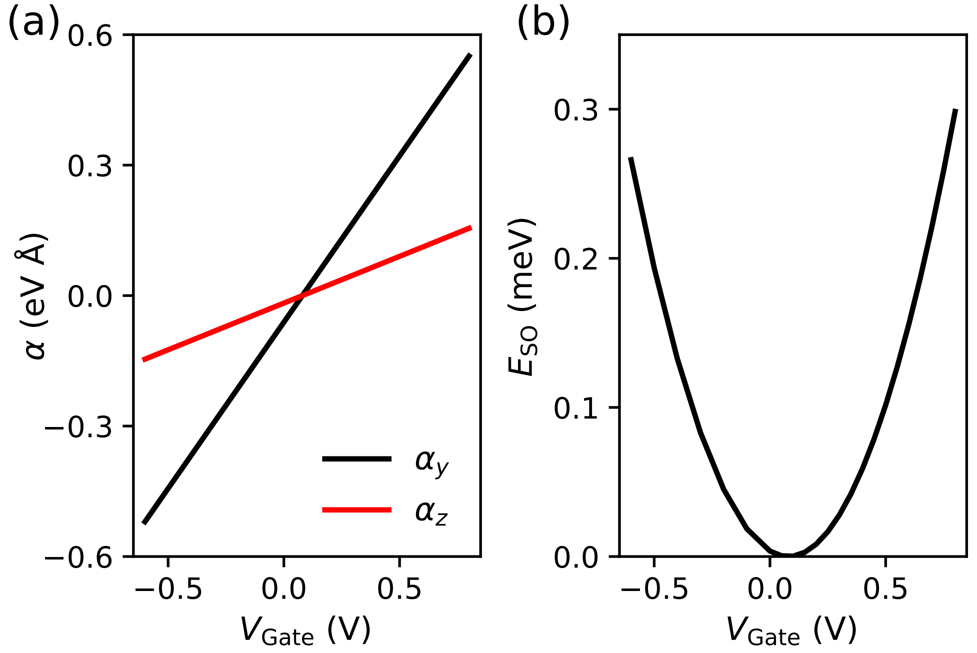


**FIG. S1:** (**a**) Rashba coefficients $\alpha_y$ and $\alpha_z$ as a function of $V_{\mathrm{Gate}}$. At $V_{\mathrm{Gate}} = 0.08\,\mathrm{V}$, the average electric field in the wire goes to zero due to symmetry, leading to vanishing spin-orbit coupling. (**b**) Calculated $E_{\mathrm{SO}}$ as a function of $V_{\mathrm{Gate}}$.

We define the spin-orbit energy $E_{\mathrm{SO}} = \frac{m^*(\alpha_y^2+\alpha_z^2)}{2\hbar^2}$. The spin-orbit energy is plotted as a function of $V_{\mathrm{Gate}}$ in Fig. S1(b). The average electric field in the nanowire increases as the applied gate voltage becomes more negative, leading to an enhancement of the spin-orbit coupling. At $V_{\mathrm{Gate}} = 0.08\,\mathrm{V}$, the average electric field in the nanowire becomes equal to 0 due to symmetry, eliminating the influence of spin-orbit coupling on the nanowire spectrum.

## S3. SIMULATED BAND STRUCTURE

The band structure of the superconductor-semiconductor nanowire system for different values of $V_{\mathrm{Gate}}$ is shown in Fig. S2. To quantify the coupling of a given state to the superconductor, we calculate the weight of the state in the semiconducting region SM (see Fig. 1(c)) as $W_{\mathrm{SM}} = \iint_{\mathrm{SM}} |\Psi(k_{\mathrm{F}})|^2 \, dy \, dz$.

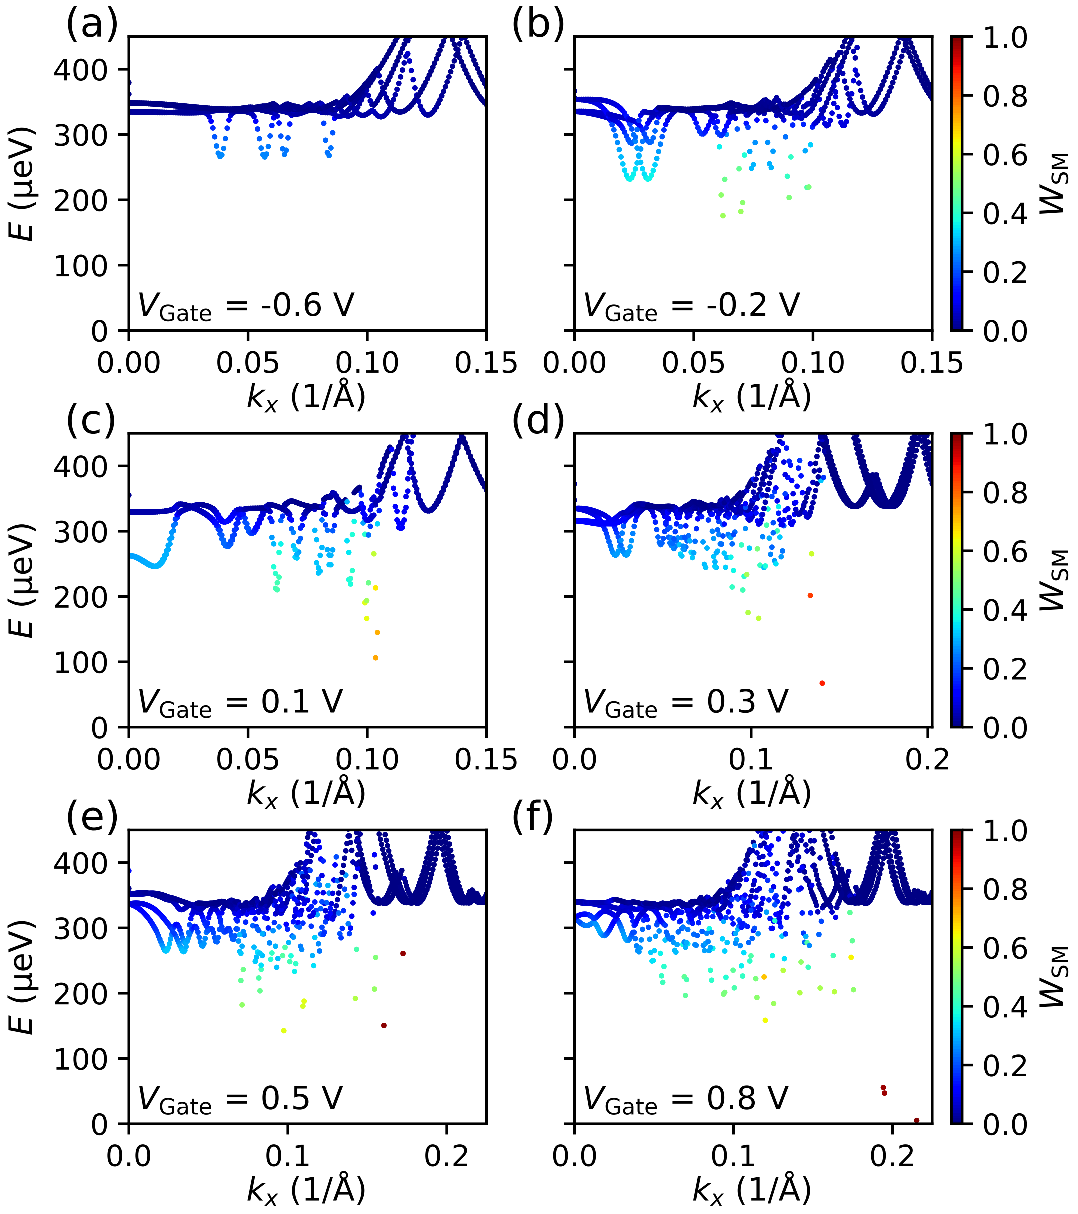


**FIG. S2:** Band structure of the hybrid system calculated at $B = 0\,\mathrm{T}$ for different values of $V_{\mathrm{Gate}}$. The color indicates the weight of a given state in the semiconducting region. As the gate voltage is increased, the population of states with higher $W_{\mathrm{SM}}$ leads to a soft gap.

## S4. FABRICATION PROCEDURE

1. **Nanowire deposition**: a SEM-based nanomanipulator is used to deterministically place the InSb-Al nanowires unto a degenerately p-doped Si substrate covered by 20 nm of LPCVD $Si_3N_4$ (devices A, C, and D) or 285 nm of thermal $SiO_2$ (device B).

2. **Mask preparation & lithography**: for every fabrication step, we use standard electron beam lithography techniques to create the mask. The mask consists of a layer of PMMA 950KA6 spun at 4000 rpm. After writing, the mask is developed in a solution of MIBK:IPA (1:3 ratio) for 60 s, followed by a IPA rinse for 60 s. After each deposition step, liftoff is done using acetone.

3. **Contact preparation & deposition**: before depositing the contact material, the Al and $AlO_x$ are locally removed by Ar plasma etch. The contacts are deposited by electron beam evaporation of Cr/Au (10/100-200 nm). For device B, the side gates are also evaporated in this step.

4. **Dielectric deposition**: as a top gate dielectric we sputter 35 nm of $SiN_x$ (devices A, C, and D).

5. **Top gate deposition**: the top gates are deposited by electron beam evaporation of Ti/Au (10/200 nm) (devices A, C, and D).

## S5. DEVICE INFORMATION AND SCHEMATICS

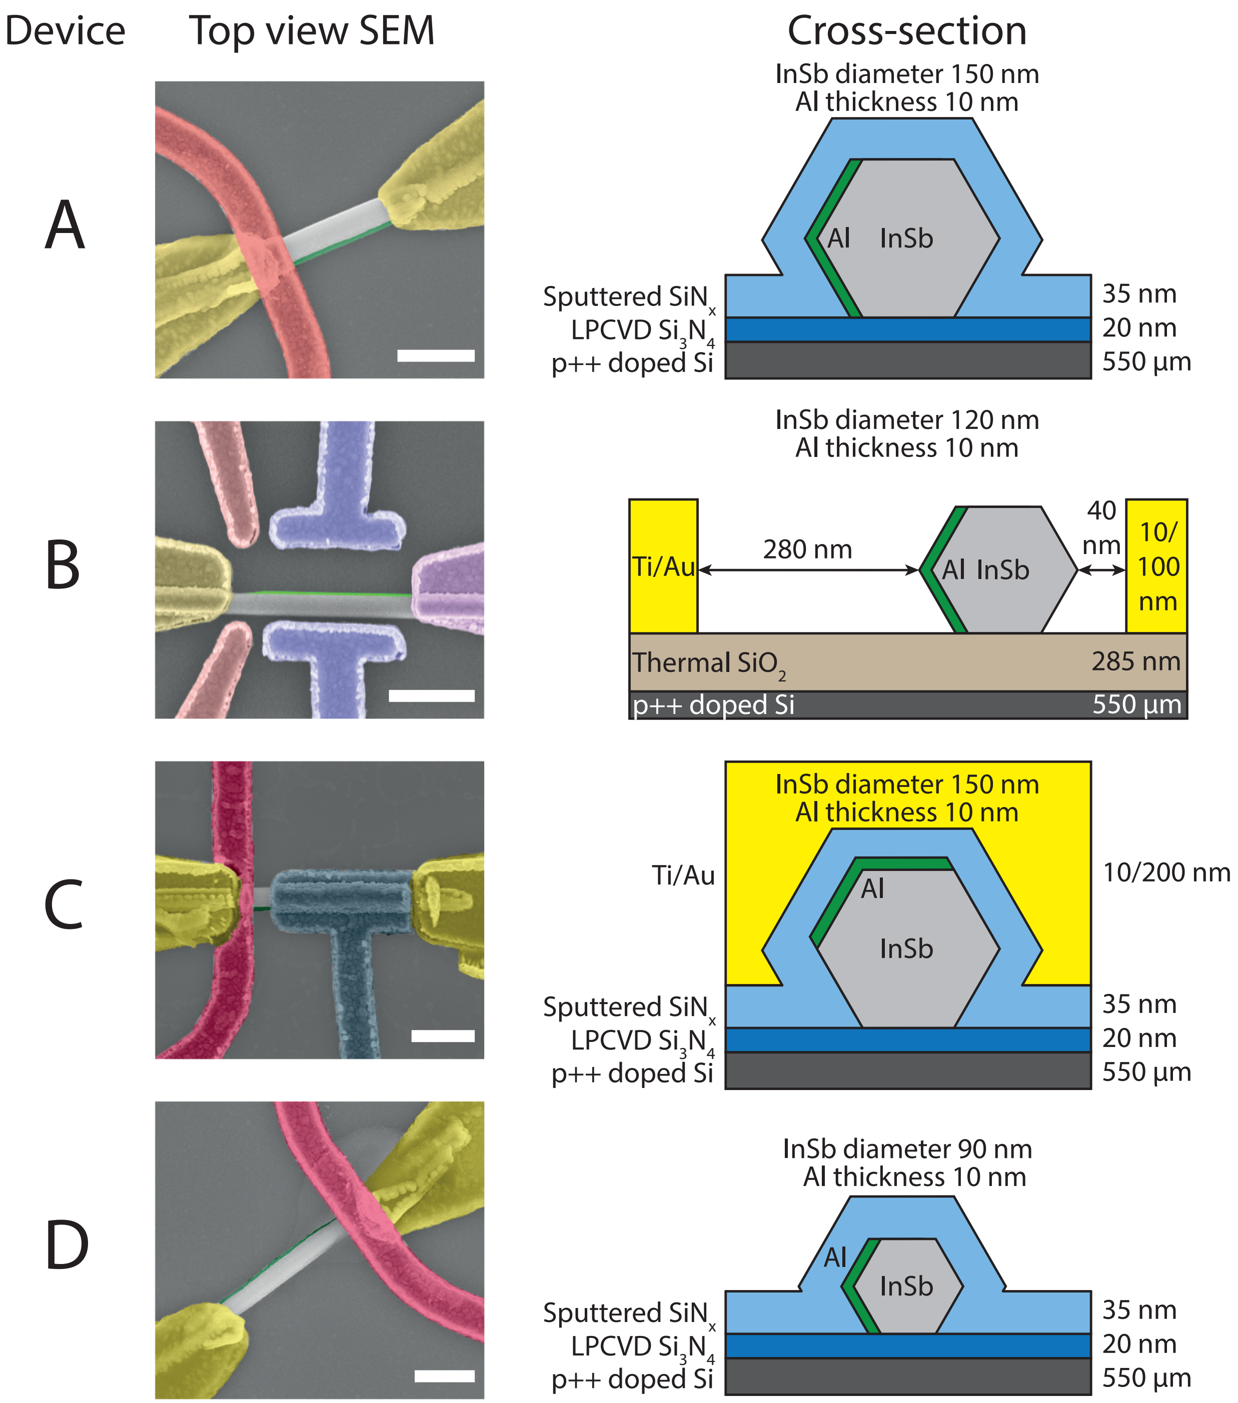


**FIG. S3:** SEM images and schematic cross-sectional views of the devices used as part of this research. Data from devices A and B is presented in the main text. Data from devices C and D is presented in the supplement for completeness. Note that the data for device B is obtained by changing the voltage on the side gate ($V_{SG}$), shown in blue in the SEM image. Scale bar is 500 nm.

## S6. GAP FITTING & ADDITIONAL DATA

To extract the gap, we measure the differential conductance $\mathrm{d}I/\mathrm{d}V$ as a function of $V_{\mathrm{Bias}}$ and tunnel gate voltage $V_{\mathrm{Tunnel}}$ for different back gate voltages $V_{\mathrm{BG}}$. In the tunneling limit, $\mathrm{d}I/\mathrm{d}V$ is approximately proportional to the density of states. To ensure we are in this limit, we take only the traces where the conductance at high bias ($\sim 500\,\mu$V) is between 0.03 and $0.08{\cdot}2e^2/h$. We use the BCS-Dynes expression for a dissipation broadened superconducting density of states [11] to arrive at the following expression for the conductance:

$$\frac{\mathrm{d}I}{\mathrm{d}V} = G_{\mathrm{N}}\mathrm{Re}\left\{\frac{V_{\mathrm{Bias}} - i\Gamma}{\sqrt{(V_{\mathrm{Bias}} - i\Gamma)^2 - \Delta^2}}\right\}. \tag{S7}$$

This equation is fitted to the data (separately for positive and negative bias), as shown in Fig. S4 for $V_{\mathrm{BG}} =$ -0.6 V. We take the average of the extracted gap values for different values of $V_{\mathrm{Tunnel}}$, with the errorbar given by the standard deviation (results plotted in Fig. 2(e)).

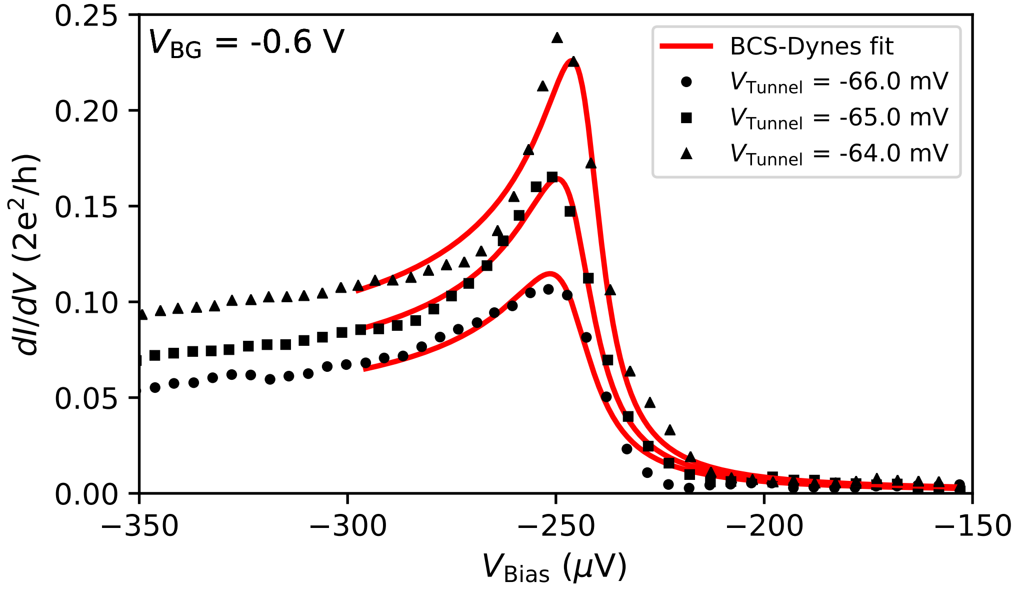


**FIG. S4:** Fit (red line) of equation (S7) to conductance data from device A (black circles, squares and triangles) for different values of the tunnel gate voltage.

Device B shows similar behavior to device A: as the side gate voltage is increased, the observed gap becomes smaller (as illustrated in Fig. S5).

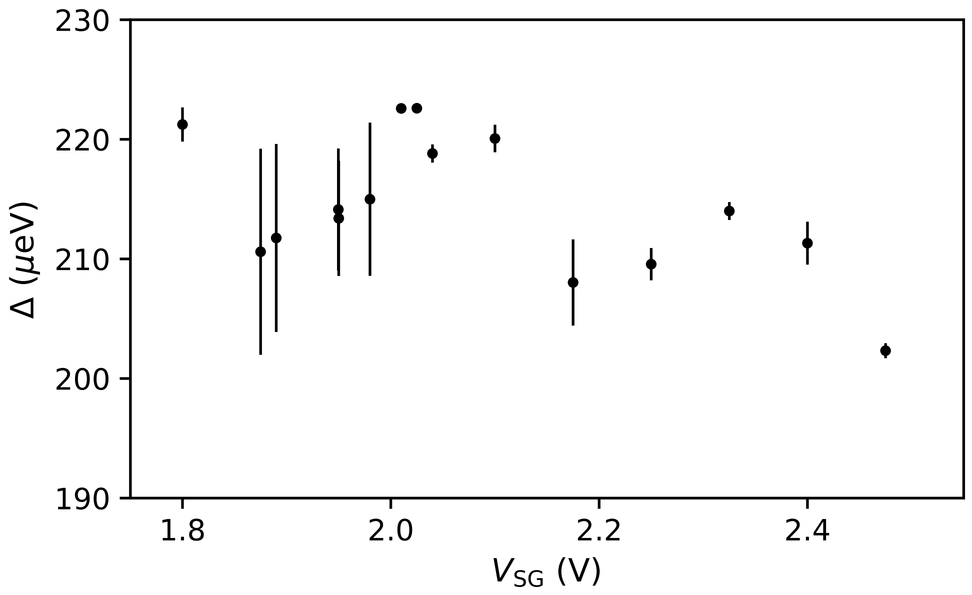


**FIG. S5:** Extracted gap $\Delta$ as a function of $V_{SG}$ for device B.

In Fig. S6, we show differential conductance traces as a function of $V_{Bias}$ in device D for different values of the back gate voltage. The voltage on the tunnel gate is chosen such that the transmission through the junction (parameterized by $G_N$) is constant.

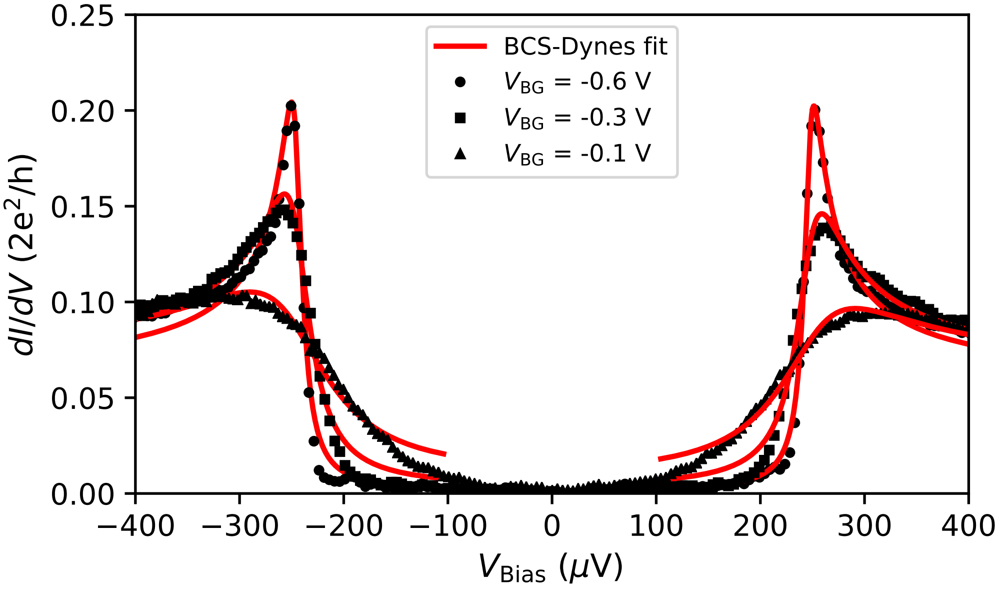


**FIG. S6:** Fit (red line) of equation S7 to conductance data from device D (black circles, squares and triangles) for different $V_{BG}$ at similar junction transparencies. The dissipation broadening sharply decreases for more negative gate voltages.

Although the sub-gap conductance is similar for all three gate voltages, there is a strong

broadening of the coherence peak as the gate voltage becomes more positive. This broadening is associated with dissipation due to an increase in the number of quasiparticles, caused by pair breaking in the superconductor. We plot the extracted gap $\Delta$ and dissipation broadening $\Gamma$ in Fig. S7.

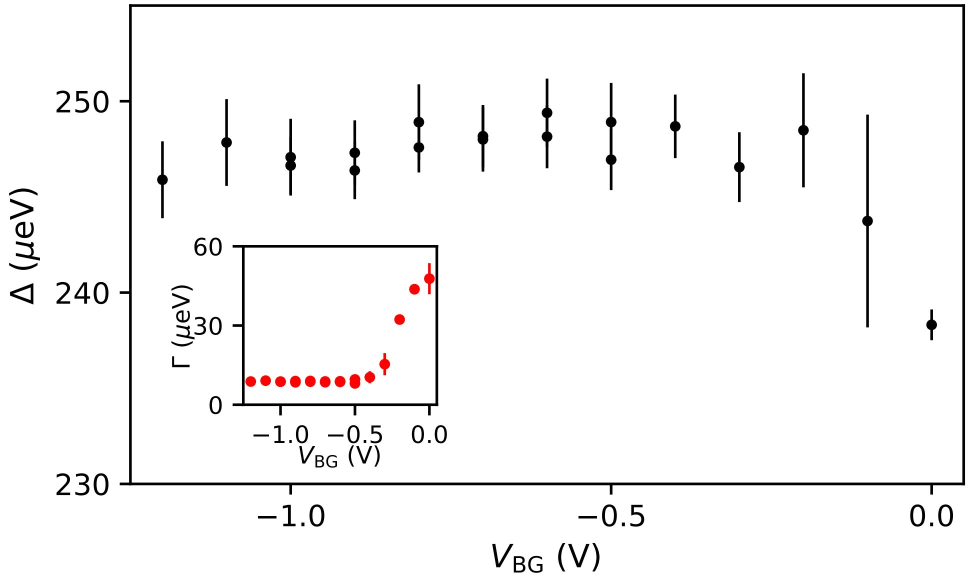


**FIG. S7:** Extracted gap $\Delta$ as a function of $V_{\mathrm{BG}}$ for device D. Inset: dissipation broadening $\Gamma$ as a function of $V_{\mathrm{BG}}$. A decrease in the gap is accompanied by an increase in broadening, signalling the emergence of a soft gap.

As in the other devices, the gap decreases for more positive gate voltages, although in this case the effect is minor. The size of the gap is quite stable over an extended range in gate voltage. We speculate that this is related to the diameter of the wire, which is smaller than in the other devices. The reduced thickness means the superconductor can screen the gate voltage more effectively throughout the wire diameter, reducing the effect of the gate on the superconductor-semiconductor coupling.

## S7. G-FACTOR FITTING & ADDITIONAL DATA

For each back gate voltage, we measure the d$I$/d$V$ as a function of $V_{\text{Bias}}$ and the magnetic field $B$. We then identify the lowest energy peak in the spectrum. The position of this peak at a given field is obtained by a peak finding algorithm, the results of which are shown as the green circles in Fig. S8. The slope $\frac{\Delta E}{\Delta B}$ is determined by a linear fit (dashed black line in Fig. S8). From the slope, we get $g_{\text{eff}}$ by using the relation $\Delta E = \frac{1}{2} g_{\text{eff}} \mu_{\text{B}} \Delta B$ for a spin-$\frac{1}{2}$ particle, with $\mu_{\text{B}}$ the Bohr magneton. This procedure is performed separately for positive and negative bias. The reported $g_{\text{eff}}$ is then calculated as a weighted average of the absolute value of the positive and negative bias results (weights determined by the variance of the fit parameters).

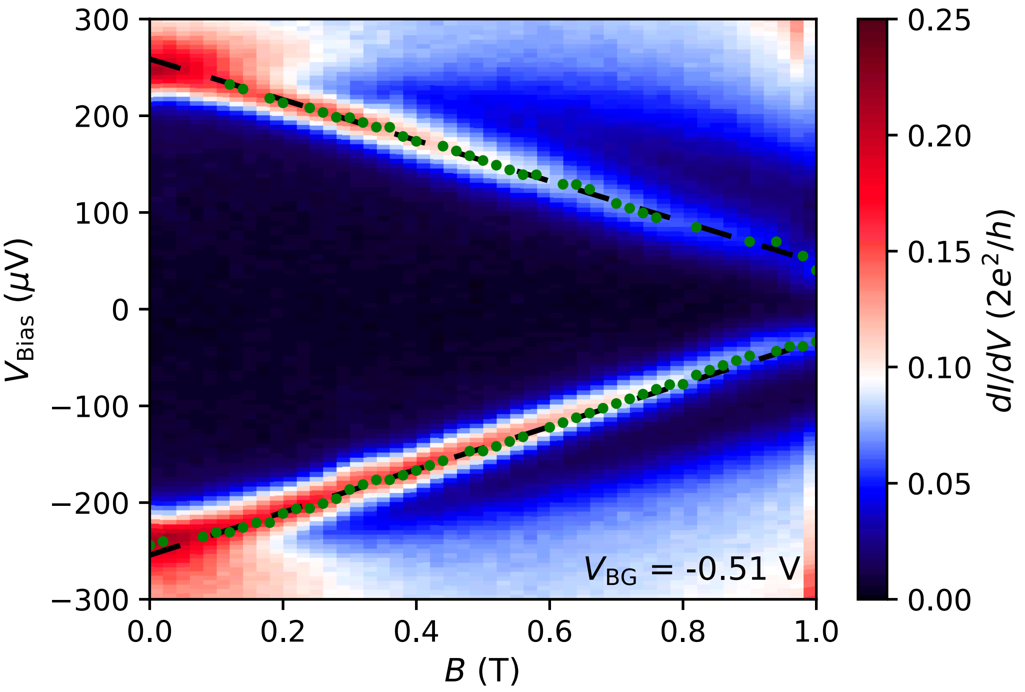


**FIG. S8:** Differential conductance as a function of $V_{\text{Bias}}$ and magnetic field. We apply a linear fit (dashed black lines) to the extracted peak positions (green circles) to obtain the average slope $\frac{\Delta E}{\Delta B}$.

The effective g-factor for device A is reported in the main text (Fig. 3(c) and Fig. 4(d), respectively). In Fig. S9, we plot the extracted g-factors of both $L_1$ and $L_2$ in device B. For completeness, data from device C is shown in Fig. S10.

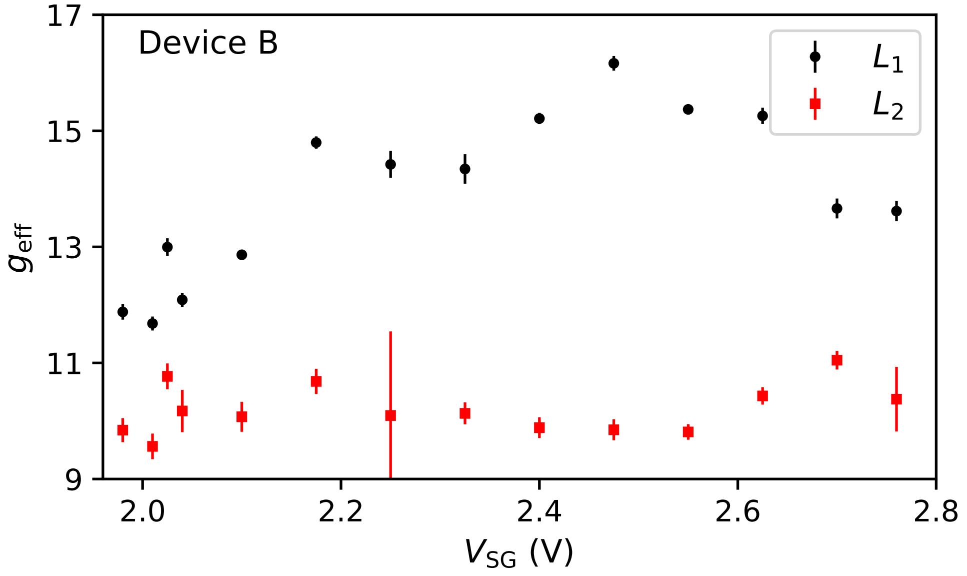


**FIG. S9:** Extracted values of $g_{\rm eff}$ as a function of $V_{\rm SG}$ for $L_1$ (black circles) and $L_2$ (red squares) in Device B.

The effective g-factor of $L_1$ (black circles) changes appreciately when the side gate voltage is changed, with the effect comparable to the one observed in device A. In contrast, $g_{\rm eff}$ of $L_2$ (red squares) is almost unaffected by the gate and has a lower value. This may be due to $L_2$ being closely confined near the superconductor, leading to a decreased g-factor due to stronger hybridization, and a weaker gate response due to enhanced screening.

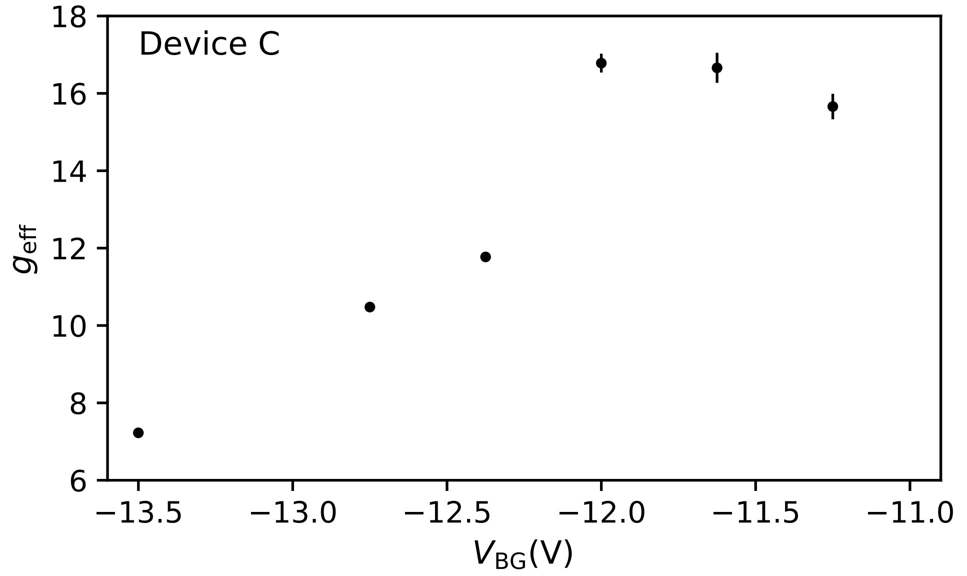


**FIG. S10:** Extracted values of $g_{\rm eff}$ for Device C.

To determine the importance of orbital effects, we calculate the nanowire spectrum as a function of magnetic field including this effect (Figs. S11(a),(b)). The orbital effect leads to an increase of the extracted values of $g_{\mathrm{eff}}$ and $g_{\mathrm{spin}}$ (Fig. S11(c)). Note that the definition of $g_{\mathrm{spin}}$ used in the main text is no longer valid when the orbital effect is included. Nevertheless, for consistency we apply the same procedure. As we do not observe these high g-factors in any of our devices, we conclude that the orbital effect does not give a significant contribution to the observed changes of $g_{\mathrm{eff}}$ with the gate voltage.

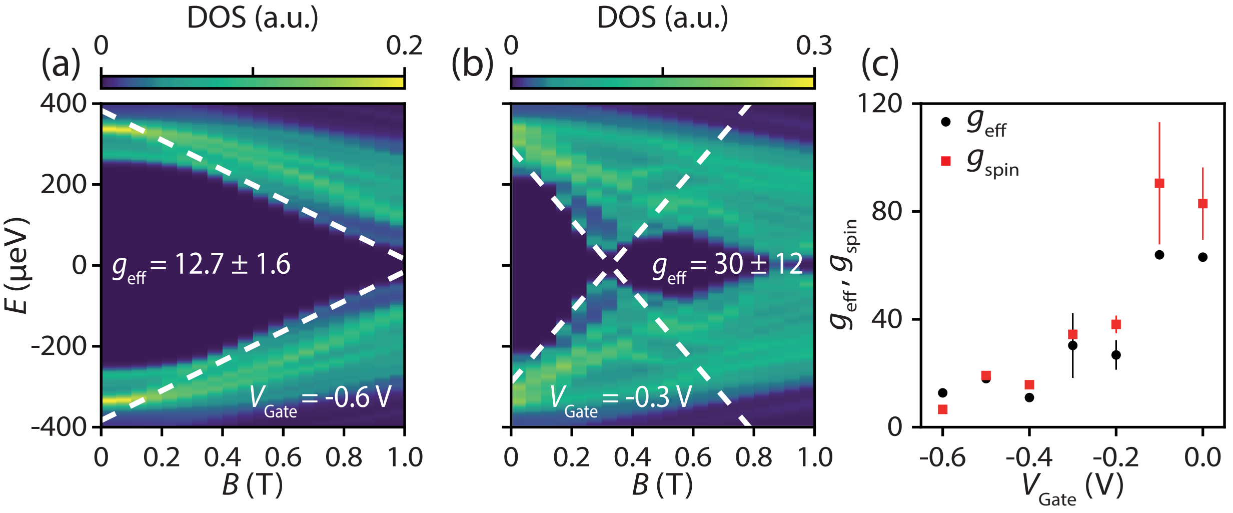


**FIG. S11:** (**a**,**b**) Simulated nanowire spectrum as a function of magnetic field including orbital effects. (**c**) Extracted $g_{\mathrm{eff}}$ (black circles) and $g_{\mathrm{spin}}$ (red squares) as a function of $V_{\mathrm{Gate}}$.

## S8. ANTICROSSING FITTING

Near the anticrossing, we approximate the energy of the lowest subgap state $L_1$ as $E_1 + \frac{1}{2}g_1\mu_\mathrm{B}B + aB^2$. The linear term represents the Zeeman contribution to the energy, while the quadratic term is a correction to account for the curvature at high fields. This is possibly due to the presence of additional levels interacting with $L_1$ in this field range. As the dispersion of $L_2$ is mostly linear in the field range of interest, we approximate it as $E_2 - \frac{1}{2}g_2\mu_\mathrm{B}B$. Adding the coupling parameter $\delta_\mathrm{SO}$, we find the energy levels of the coupled system from the eigenvalues of the matrix

$$\begin{bmatrix} E_1 + \frac{1}{2}g_1\mu_\mathrm{B}B + aB^2 & \delta_\mathrm{SO} \\ \delta_\mathrm{SO} & E_2 - \frac{1}{2}g_2\mu_\mathrm{B}B \end{bmatrix}.$$

By fitting the expression for the eigenvalues to the data, we extract the parameters $E_{1,2}$, $g_{1,2}$, $a$, and $\delta_\mathrm{SO}$. To prevent overfitting, we use estimates for the uncoupled asymptotes to constrain the fit parameters. From the obtained parameters we also calculate the splitting $A$, defined as the maximum deviation from zero energy of the lowest energy state $L_1$, after the first zero energy crossing has occurred.

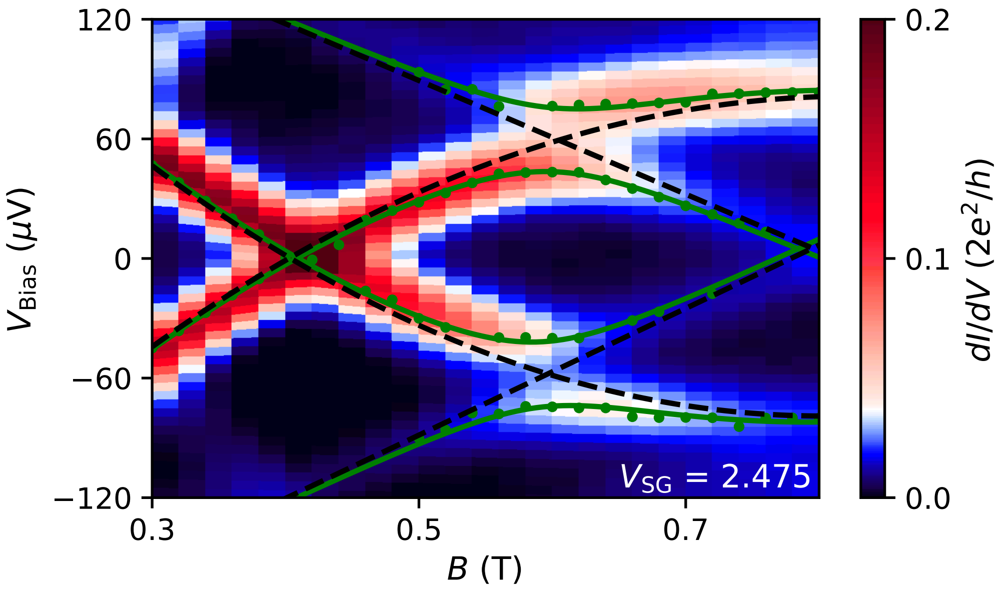


**FIG. S12:** Data from device B, showing the differential conductance $\mathrm{d}I/\mathrm{d}V$ as a function of $V_\mathrm{Bias}$ and $B$ for $V_\mathrm{BG} = 2.475\,\mathrm{V}$. Green dots indicate the peak positions found using a peak finding algorithm. The fit to the data is shown in green, with the uncoupled asymptotes as the black dashed lines.

## S9. SIMULATION OF FINITE SIZE NANOWIRE SYSTEM

To simulate the finite nanowire system, we solve the Hamiltonian (S5) in a simplified setup. We consider a rectangular cross-section in the $yz$-plane similar to the one used in ref. [2], where the top facet of the rectangle is covered by the superconductor, and a uniform gate voltage $V_{\mathrm{Gate}}$ is applied to the bottom facet, as illustrated in Fig. S13. First, we assume an infinitely long nanowire oriented in the $x$-direction, and calculate the electrostatic potential in the Thomas-Fermi approximation, similar to the procedure described in S1. The fermi level in the nanowire is tuned such that it supports the same number of transverse modes at $V_{\mathrm{Gate}} = 0$ as the hexagonal nanowire studied previously. We use the same material parameters as in the previous simulation, which can be found in table SI.

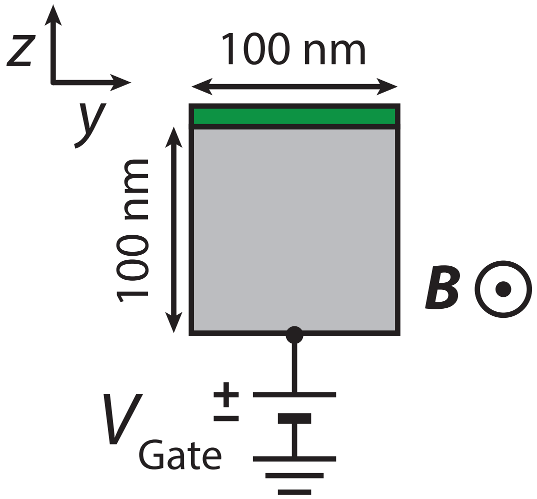


**FIG. S13:** Schematic cross-section of the geometry used to simulate the finite nanowire system. A potential $V_{\mathrm{Gate}}$ is applied to the bottom facet, while the potential at the top facet is fixed by the work function difference between the two materials. The magnetic field is applied in the $x$-direction, along length of the nanowire.

We then plug the resulting electrostatic potential into S5 and solve the Schrödinger equation to find the low energy spectrum of the finite nanowire. We take a length of 750 nm, similar to the studied devices. We calculate only the modes in the semiconductor, assuming a superconducting gap of $\Delta = 250\,\mu$eV. We find that the origin of the level repulsion between states is indeed spin-orbit coupling, which couples different longitudinal (along the $x$-direction) states within the same transverse ($y$- and $z$-directions) subband.

The result is illustrated in Fig. S14, where we plot the low energy spectrum as a function of Zeeman energy $E_Z$ for a fixed value of $V_{Gate}$ and different values of $\alpha$. An increase in the spin-orbit coupling strength leads to an increase in the level repulsion.

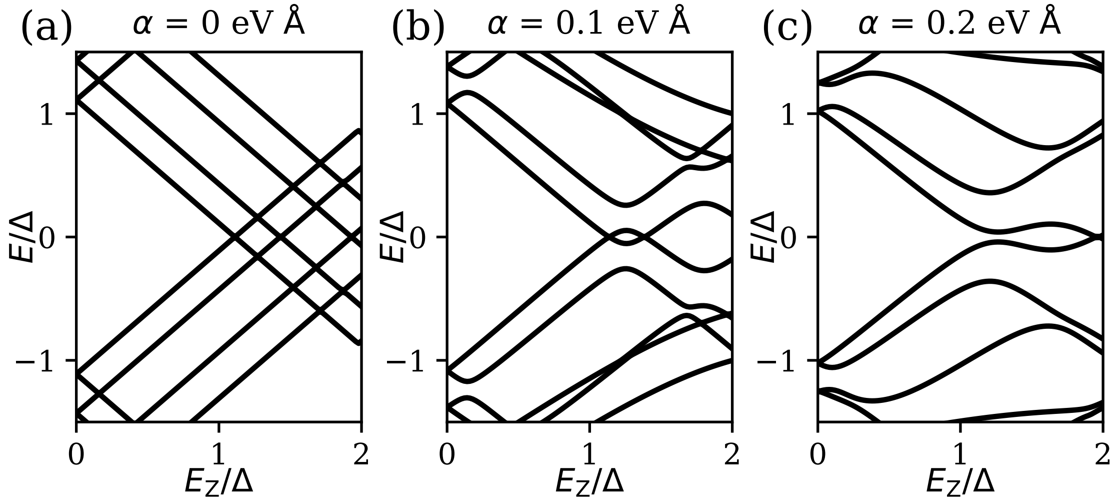


**FIG. S14:** Calculated low energy spectrum of the finite size nanowire as a function of Zeeman energy for different values of $\alpha$. Values calculated for $V_{Gate}$ = -0.536 V, which is also used in main text Fig. 4(d). All energy scales are in units of the superconducting gap $\Delta$.

However, even if $\alpha$ is fixed, the magnitude of the level repulsion can be changed by changing the confinement potential, as demonstrated in Fig. S15.

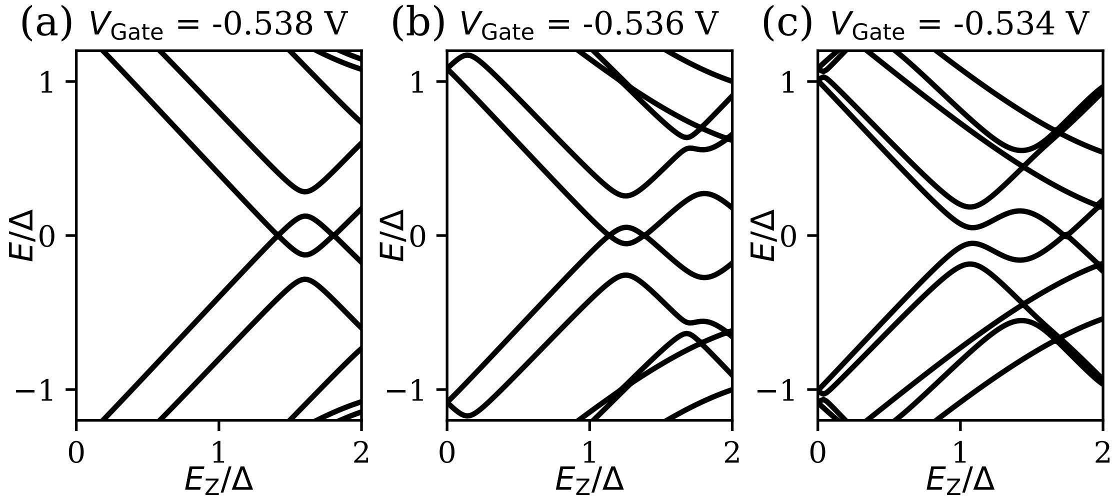


**FIG. S15:** Calculated low energy spectrum of the finite size nanowire as a function of Zeeman energy for different values of $V_{Gate}$. Values calculated $\alpha = 0.1$ eV Å, energy scales in units of $\Delta$.

When the gate voltage is changed, it alters the confinement potential. This affects the energy of the levels coupled by the spin-orbit coupling, and as such directly influences the magnitude of $\delta$, even though the spin-orbit coupling strength itself is not changed appreciatively. In Fig. S16 we plot the calculated energy gap due to level repulsion, $2\delta$, and the maximum splitting from zero energy of the lowest energy state after the first zero crossing, $A$, as a function of $V_{\mathrm{Gate}}$. The two parameters follow opposite trends, consistent with the experimental observation in Fig. 4(f).

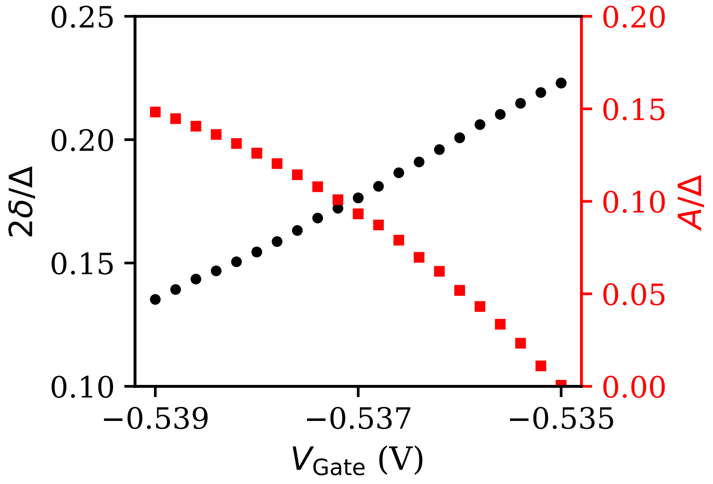


**FIG. S16:** Dependence of the energy gap $2\delta$ and the splitting $A$, in units of $\Delta$, on the gate voltage $V_{\mathrm{Gate}}$.

However, the trend with gate voltage is opposite: $\delta$ increases with more positive gate voltage, whereas in the experiment it decreases. We note that the geometry used in this simulation is a simplified version of the one used in the experiment. The dependence of the confinement energy on gate voltage is strongly dependent on the geometry, which differs between the simulation and the experiment. It is therefore expected that the trend of $\delta$ with gate voltage is not universal, and requires the details of the systems to be very similar before comparisons can be made.

## S10. ADDITIONAL ZBP DATA

Fig. S17(a) shows the differential conductance measured in device A as a function of $V_{\mathrm{Bias}}$ and $V_{\mathrm{Tunnel}}$, for $B$ = 0.35 T and $V_{\mathrm{BG}}$ = -0.37 V. The low energy spectrum in this parameter regime does not depend on the transmission of the NS-junction. In Fig. S17(b), we show line traces for different values of $V_{\mathrm{Tunnel}}$. Even though the transmission of the junction is changed by a factor of two, the peak position of the low energy states are not affected. Data from main text Fig. 5 was obtained for $V_{\mathrm{Tunnel}}$ = -87 mV.

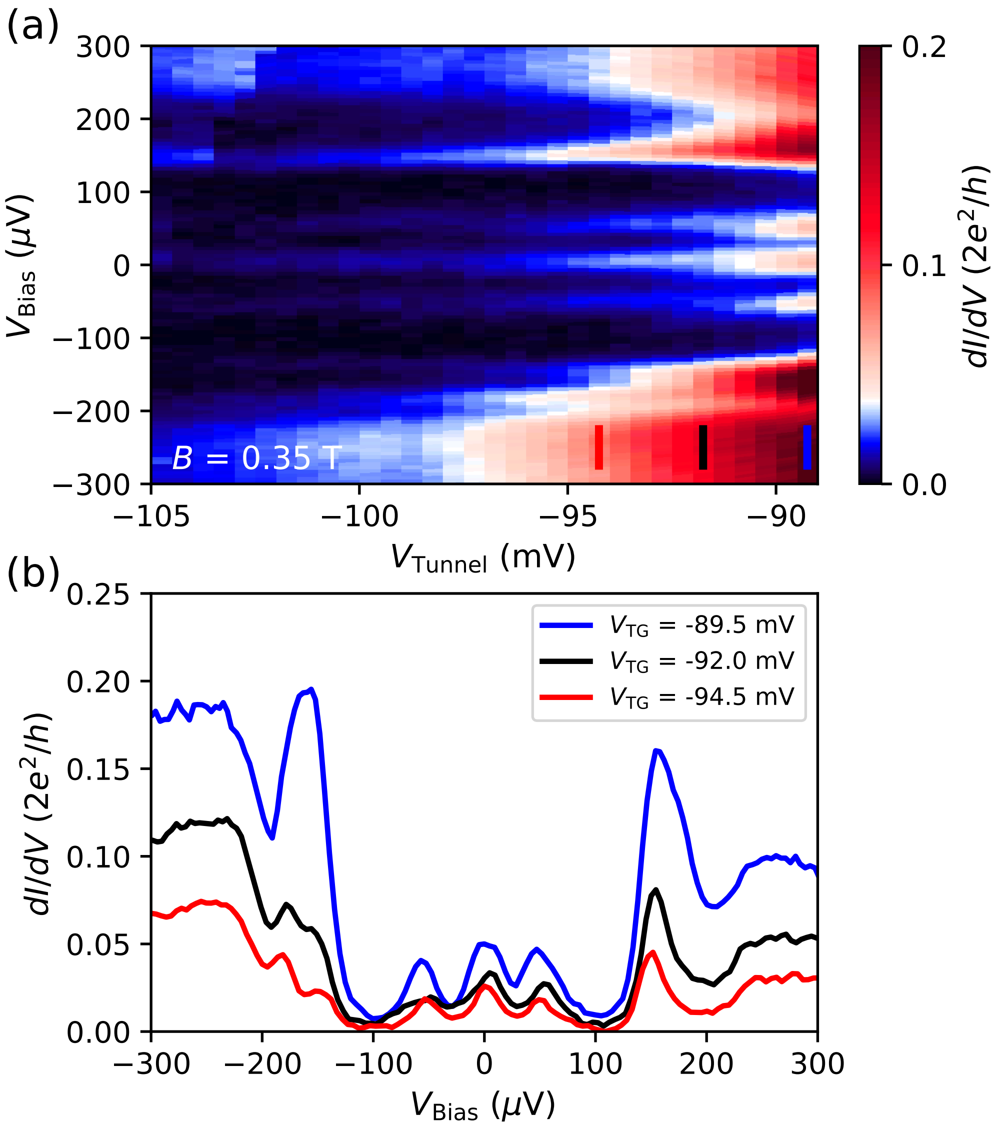


**FIG. S17:** (**a**) d$I$/d$V$ measured in device A as a function of $V_{\mathrm{Bias}}$ and $V_{\mathrm{Tunnel}}$ for $B$ = 0.35 T and $V_{\mathrm{BG}}$ = -0.37 V. (**b**) Line traces at the values of $V_{\mathrm{Tunnel}}$ indicated by the colored lines in panel (a).

Figure S18 shows additional data on the evolution of the level repulsion between $L_1$ and $L_2$ in device A (supplementing the data presented in main text Figs. 5(a-c)) as the back gate voltage is increased. As discussed in the main text, we do not find an extended region in parameter space with a stable zero bias conductance peak.

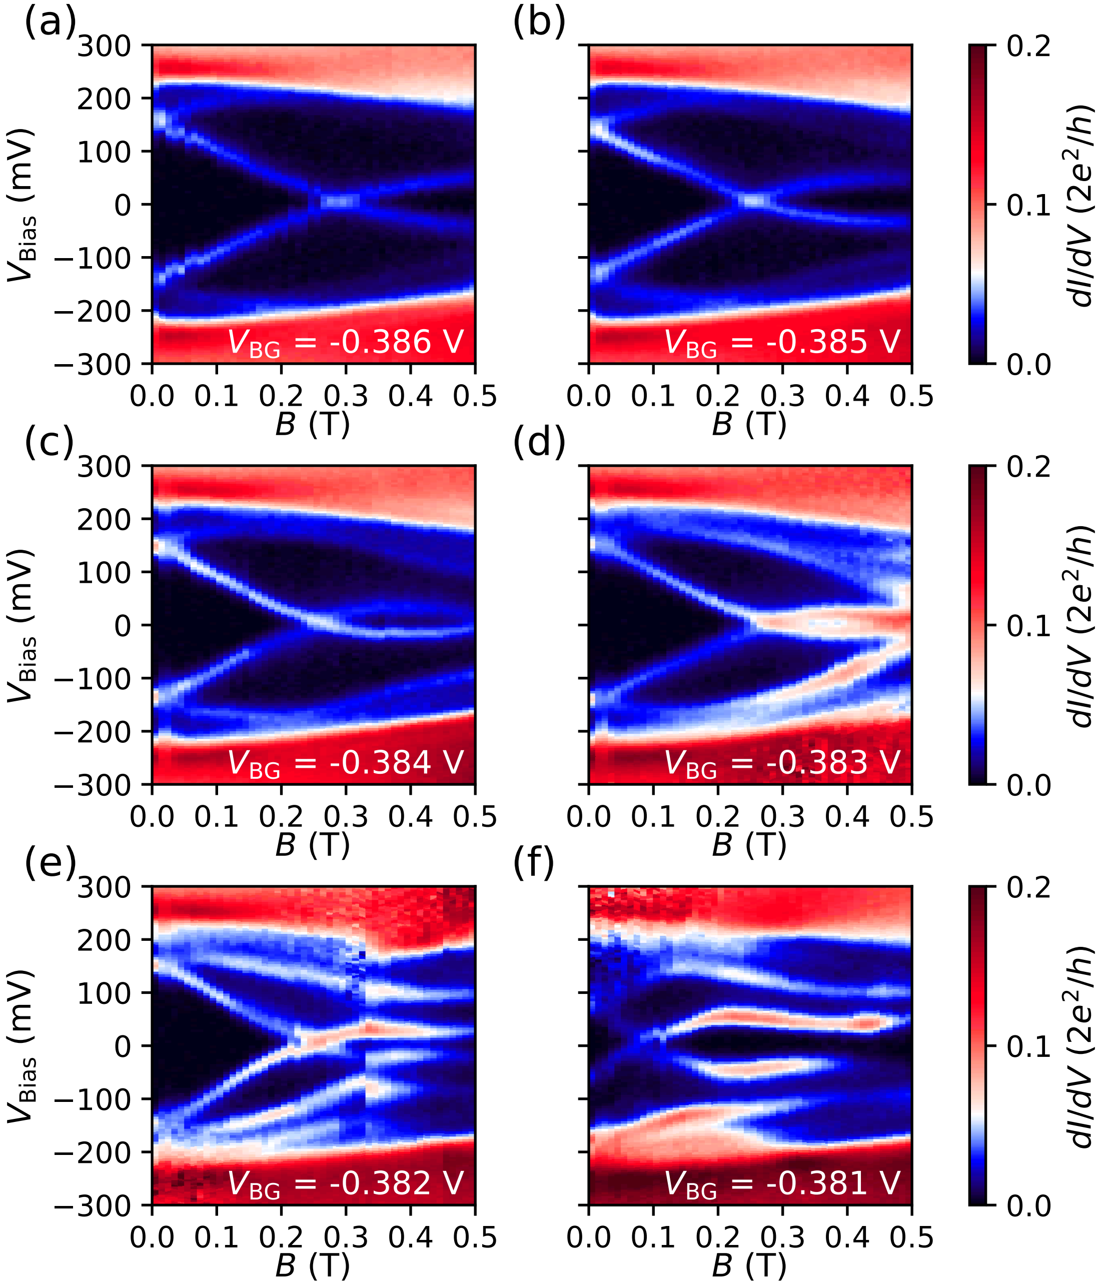


**FIG. S18:** Differential conductance as a function of $V_{\mathrm{Bias}}$ and magnetic field. Although the lowest energy state stays near zero over an extended magnetic field range for some gate voltages, this behavior is not robust.

In Fig. S19 we show the low energy spectrum of device A as a function of $V_{\text{Bias}}$ and $V_{\text{BG}}$ for different magnetic fields (supplementing the data presented in main text Figs. 5(e,f)). For specific combinations of magnetic field and gate voltage, we can find a zero energy state. However, as we do not find an extended region in parameter space, it is unlikely that a topological phase transition is responsible for this observation.

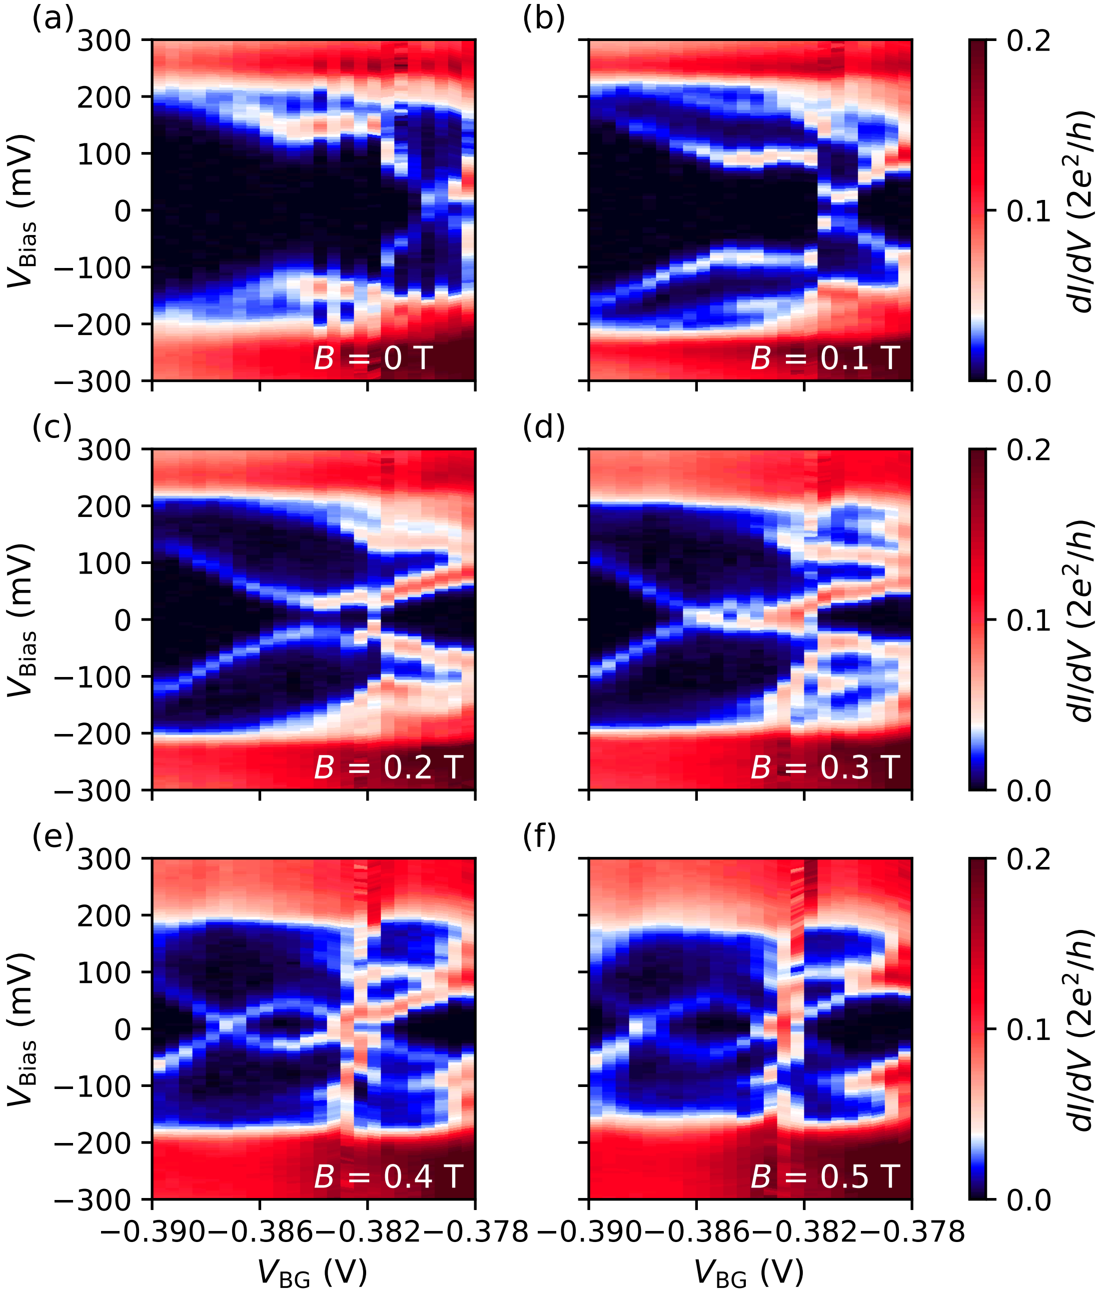


**FIG. S19:** Differential conductance as a function of $V_{\text{Bias}}$ and $V_{\text{BG}}$. We find some stable ZBPs for certain ranges in back gate voltage at specific fields, but this is only true for fine tuned parameters.

[1] R. Winkler, S. J. Papadakis, E. P. De Poortere, and M. Shayegan, *Spin-Orbit Coupling in Two-Dimensional Electron and Hole Systems*, Vol. 41 (Springer, 2003).

[2] A. E. Antipov, A. Bargerbos, G. W. Winkler, B. Bauer, E. Rossi, and R. M. Lutchyn, "Effects of gate-induced electric fields on semiconductor Majorana nanowires," (2018), arXiv:1801.02616.

[3] S. R. Plissard, I. van Weperen, D. Car, M. A. Verheijen, G. W. G. Immink, J. Kammhuber, L. J. Cornelissen, D. B. Szombati, A. Geresdi, S. M. Frolov, L. P. Kouwenhoven, and Bakkers E. P. A. M., "Formation and electronic properties of InSb nanocrosses," Nature Nanotechnology **8**, 859–864 (2013).

[4] W. Chang, S. M. Albrecht, T. S. Jespersen, F. Kuemmeth, P. Krogstrup, J. Nygård, and C. M. Marcus, "Hard gap in epitaxial semiconductor-superconductor nanowires," Nature Nanotechnology **10**, 232–235 (2015).

[5] J. Kammhuber, M. C. Cassidy, H. Zhang, Ö. Gül, F. Pei, M. W. A. de Moor, B. Nijholt, K. Watanabe, T. Taniguchi, D. Car, S. R. Plissard, E. P. A. M. Bakkers, and L. P. Kouwenhoven, "Conductance Quantization at Zero Magnetic Field in InSb Nanowires," Nano Letters **16**, 3482–3486 (2016).

[6] R. Meservey and P. M. Tedrow, "Properties of Very Thin Aluminum Films," Journal of Applied Physics **42**, 51–53 (1971).

[7] N. Ashcroft and N. Mermin, *Solid State Physics* (Saunders College Publishing, 1976).

[8] M. Tinkham, *Introduction to Superconductivity*, Dover Books on Physics Series (Dover Publications, 1996).

[9] B. Nijholt and A. R. Akhmerov, "Orbital effect of magnetic field on the Majorana phase diagram," Phys. Rev. B **93**, 235434 (2016).

[10] C. W. Groth, M. Wimmer, A. R. Akhmerov, and X. Waintal, "Kwant: a software package for quantum transport," New Journal of Physics **16**, 063065 (2014).

[11] R. C. Dynes, V. Narayanamurti, and J. P. Garno, "Direct Measurement of Quasiparticle-Lifetime Broadening in a Strong-Coupled Superconductor," Phys. Rev. Lett. **41**, 1509–1512 (1978).
